# Supplementary material for: Visual Large Language Models Exhibit Human-Level Cognitive Flexibility in the Wisconsin Card Sorting Test
Source: arXiv:2505.22112 ancillary file (2025-05-28)
Supplement: Supplementary file 1 [file Supplementary_Material.pdf]

## Supplementary Material

## "Visual Large Language Models Exhibit Human-Level Cognitive Flexibility in the Wisconsin Card Sorting Test"

### Figures


| | | Page |
|---|---|---|
| Figure s-1 | ALIEN Task Performance | 2 |
| Figure s-2 | WCST Task Description | 3 |
| Figure s-3 | WCST Prompt Description | 4 |
| Figure s-4 | ALIEN Prompt Description | 5 |
| Figure s-5 | WCST Human Experiment Interface | 6 |
| Figure s-6 | WCST Role Description | 7 |
| Figure s-7 | WCST Task Example | 8 |
| Figure s-8 | WCST Vision Example | 9 |


### Tables


| | | Page |
|---|---|---|
| Table t-1 | ALIEN Task Performance Metrics | 2 |
| Table t-2 | ALIEN Task Cost Analysis | 2 |

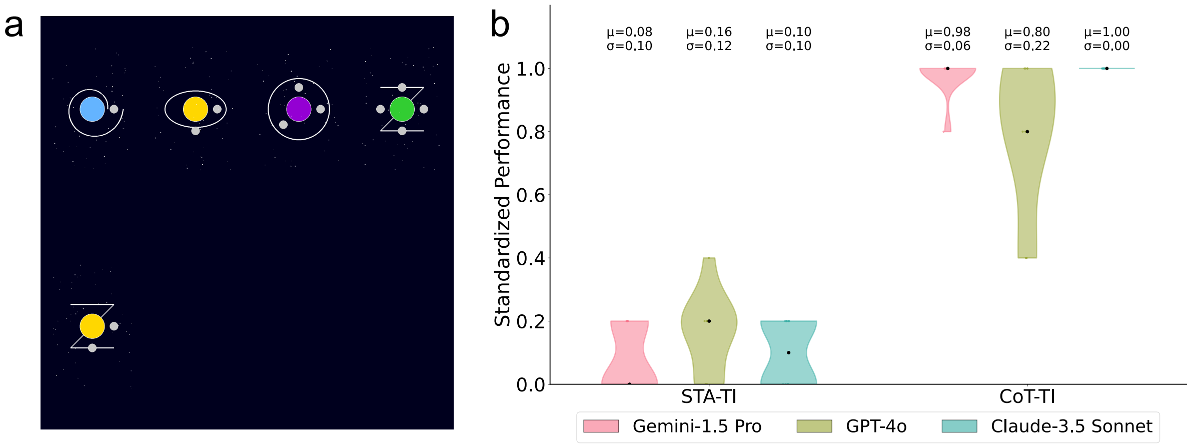


Figure s-1: **ALIEN Task Performance.** (a) The Alien Task is a variant of the WCST that retains the same logical structure but uses different terminology and framing. Instead of the original WCST dimensions, it substitutes: shape → orbit_type (spiral, elliptical, circular, Z-shaped), color → atmosphere (hydrogen, helium, nitrogen, oxygen), and count → moons (1, 2, 3, 4). This alien civilization exploration theme helps rule out the possibility that models simply recall preexisting examples from their training set. (b) Performance comparison of all models under STA-TI and CoT-TI conditions shows results consistent with the original WCST task.

Table t-1: ALIEN Task Performance Metrics Across Models and Experimental Conditions

| Model | Condition | CC | PE | NPE | TFC | CLR (%) | FMS |
|---|---|---|---|---|---|---|---|
| Gemini-1.5 Pro | STA-TI | 0.40 (0.52) | 8.30 (11.10) | 31.70 (19.05) | 17.75 (-) | 9.06 (9.31) | 0.20 (0.63) |
| | CoT-TI | 4.90 (0.32) | 5.80 (0.79) | 3.40 (2.17) | 12.40 (0.84) | 66.72 (2.95) | 0.00 (0.00) |
| GPT-4o | STA-TI | 0.80 (0.63) | 15.40 (14.08) | 15.50 (13.64) | 26.00 (-) | 20.00 (8.96) | 0.60 (0.70) |
| | CoT-TI | 4.00 (1.15) | 7.40 (3.17) | 2.70 (1.64) | 13.40 (1.65) | 61.72 (7.91) | 0.30 (0.67) |
| Claude-3.5 Sonnet | STA-TI | 0.50 (0.53) | 10.20 (12.44) | 22.00 (14.26) | 15.40 (-) | 13.91 (8.73) | 0.70 (0.82) |
| | CoT-TI | 5.00 (0.00) | 6.60 (0.97) | 1.70 (1.34) | 12.00 (1.05) | 67.19 (2.09) | 0.00 (0.00) |

Table t-2: Token Usage and Cost Analysis for ALIEN Task

| Model | Condition | Task | Last Token Avg | Session Token Avg | Session Price Avg | Total Tokens | Total Price |
|---|---|---|---|---|---|---|---|
| Gemini-1.5 Pro | STA-TI | ALIEN_TASK | 7,538 | 256,114 | $0.9 | 2,561,136 | $8.99 |
| | CoT-TI | ALIEN_TASK | 10,012 | 341,167 | $1.21 | 3,411,670 | $12.13 |
| GPT-4o | STA-TI | ALIEN_TASK | 7,915 | 268,211 | $1.34 | 2,682,112 | $13.44 |
| | CoT-TI | ALIEN_TASK | 23,728 | 790,316 | $4.12 | 7,903,163 | $41.15 |
| Claude-3.5 Sonnet | STA-TI | ALIEN_TASK | 8,684 | 293,680 | $0.89 | 2,936,802 | $8.9 |
| | CoT-TI | ALIEN_TASK | 24,208 | 797,286 | $2.58 | 7,972,855 | $25.83 |

**Task Description (Normal) :**
In this task, you will be presented with an image containing five cards. Each card has figures that differ in number, color, and shape. Four cards will be displayed at the top of the image, and one card will appear in the bottom left corner of the image. Your task will be to try to determine which of the four cards at the top the bottom left card belongs to. ***The correct answer depends upon a rule, which will be based solely on either the number of shapes, the color of the shapes, or the shape type itself.*** *There will be no combination of these characteristics to define the rule.* For example: If the rule is to match according to color, you should choose the card that matches the color of the bottom left card. If the rule is to match according to shape, you should choose the card that has the same shape as the bottom left card. If the rule is to match according to the number of shapes, you should choose the card that has the same number of shapes as the bottom left card. We will not tell you what the rule is. However, we will provide feedback after each selection, indicating only whether your selection was correct or incorrect, without any feedback into your reasoning process. The rule may change during the task. When the rule changes, you should figure out what the rule is as quickly as possible. When you make your selection, for each trial, respond ONLY in this format: Selection: [Card number, 1-4]. Example response: Selection: 2. You can just choose from the top four cards, not from the bottom left card. Feedback will be given after each selection, and you will be presented a different image. This task consists of 64 trials involving different images. Please proceed with the first image.

**Task Description ( w/o Constraints) :**
In this task, you will be presented with an image containing five cards. Each card has figures that differ in number, color, and shape. Four cards will be displayed at the top of the image, and one card will appear in the bottom left corner of the image. Your task will be to try to determine which of the four cards at the top the bottom left card belongs to. ***The correct answer depends upon a rule, which will be based solely on either the number of shapes, the color of the shapes, or the shape type itself.*** For example: If the rule is to match according to color, you should choose the card that matches the color of the bottom left card. If the rule is to match according to shape, you should choose the card that has the same shape as the bottom left card. If the rule is to match according to the number of shapes, you should choose the card that has the same number of shapes as the bottom left card. We will not tell you what the rule is. However, we will provide feedback after each selection, indicating only whether your selection was correct or incorrect, without any feedback into your reasoning process. The rule may change during the task. When the rule changes, you should figure out what the rule is as quickly as possible. When you make your selection, for each trial, respond ONLY in this format: Selection: [Card number, 1-4]. Example response: Selection: 2. You can just choose from the top four cards, not from the bottom left card. Feedback will be given after each selection, and you will be presented a different image. This task consists of 64 trials involving different images. Please proceed with the first image.

Figure s-2: **WCST Task Description.**

**Image :**

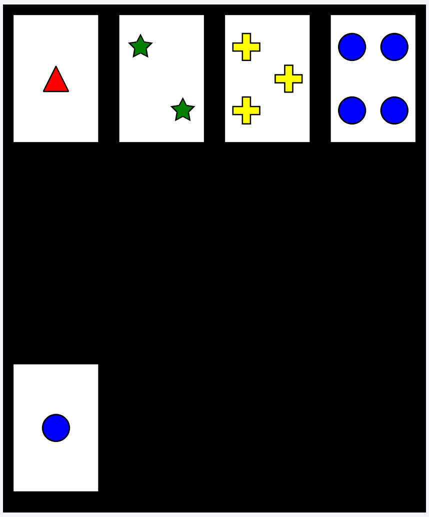

**Task Description :**

In this task, you will be presented with an image containing five cards. Each card has figures that differ in number, color, and shape. Four cards will be displayed at the top of the image, and one card will appear in the bottom left corner of the image. Your task will be to ...

**Image Description :**

The image shows four cards with white background at the top, the first card is with 1 single red triangle, the second card is with 2 green stars, the third card is with 3 yellow cross signs, the fourth card is with 4 blue circles. And there is one card at the bottom left with 1 single blue circle.

**PROMPT_TYPES**

**Straight-to-Answer (STA) :**

Provide your final answer immediately without explaining your reasoning. Your response should be concise and direct, containing only the essential information required by the task. Do not include any additional explanations or thought processes.

**Chain-of-Thought (CoT) :**

Let's think step by step, first explain your thought process in detail, then clearly state your final response to the task.

**VISION_QUESTION**

First, state how many cards you see in the image. Then, describe each card in detail. The cards contain shapes that vary in color, type, and number. For each card, provide the following information: number of shapes, color of shapes, and shape type. Format your response as: Number of cards: [number], Card Label: [number, color, shape], ...

Figure s-3: **WCST Prompt Description.**

**Task Description (Normal) :**
In this task, you will be presented with an image showing five planets from different star systems. Four reference planets will be displayed at the top of the image, and one planet will appear in the bottom left corner. Your task is to determine which of the four reference planets the bottom left planet belongs with. ***The correct answer depends on a classification rule based solely on either the planet's orbit type, atmospheric composition (represented by the planet's color), or number of moons.*** *There will be no combination of these characteristics to define the rule.* For example: If the rule is to classify according to atmosphere, you should choose the reference planet that has the same atmospheric composition (same color) as the bottom left planet. If the rule is to classify according to orbit type, you should choose the reference planet that has the same orbit pattern. If the rule is to classify according to moons, you should choose the reference planet that has the same number of moons. We will not tell you what the rule is. However, we will provide feedback after each selection, indicating only whether your classification was correct or incorrect, without explaining why. The rule may change during the task. When the rule changes, you should determine the new rule as quickly as possible. When making your selection for each trial, respond ONLY in this format: Selection: [Planet number, 1-4]. Example response: Selection: 2. You can only choose from the four reference planets at the top. Feedback will be given after each selection, and you will be presented with a different image. This task consists of 64 trials involving different planetary systems. Please proceed with the first image.

**Image :**

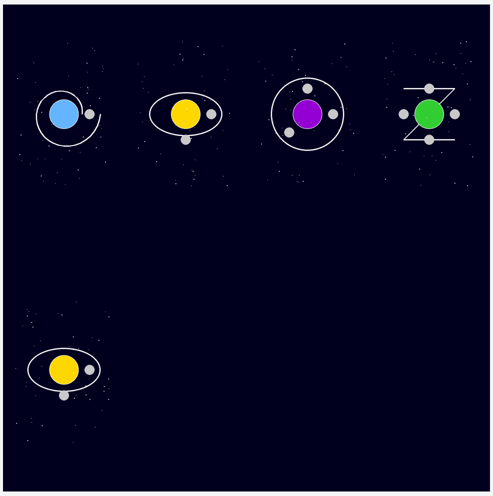

**Task Description :**
In this task, you will be presented with an image showing five planets from different star systems. Four reference planets will be displayed at the top of the image, and one planet will appear in the bottom left corner. Your task is to determine which of the four ...

**Image Description :**
The image shows four reference planets at the top: the first has a spiral orbit with hydrogen atmosphere and 1 moon, the second has an elliptical orbit with helium atmosphere and 2 moons, the third has a circular orbit with nitrogen atmosphere and 3 moons, the fourth has a z-shaped orbit with oxygen atmosphere and 4 moons. At the bottom left is a planet with elliptical orbit, helium atmosphere, and 2 moons.

Figure s-4: **ALIEN Prompt Description.**

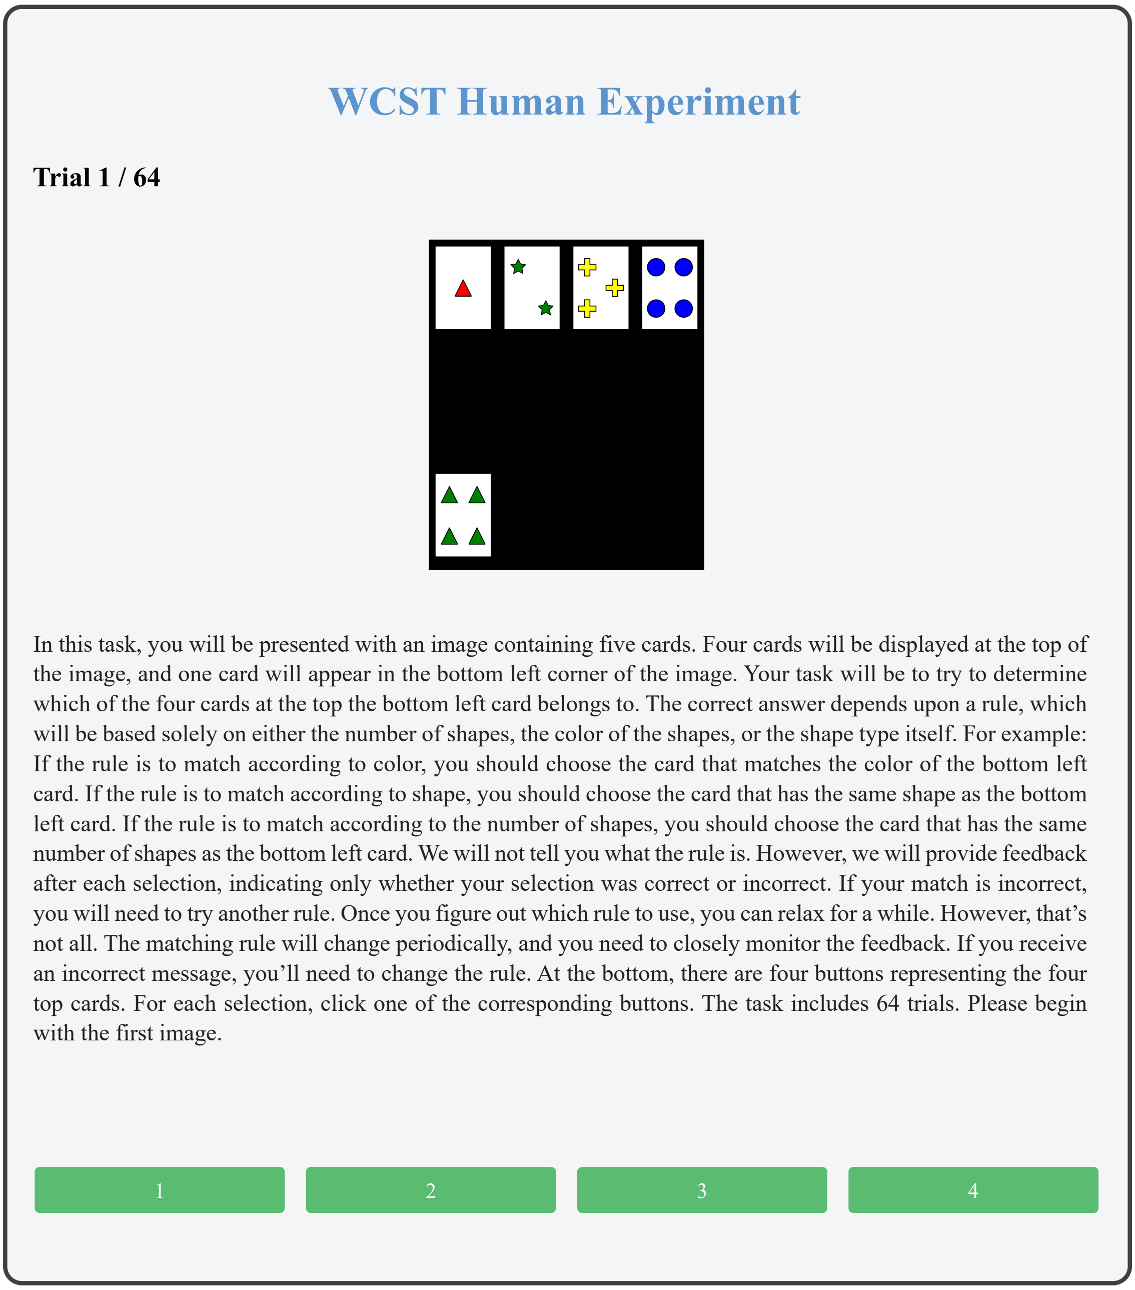


Figure s-5: **WCST Human Experiment Interface.**

**ROLE_DESCRIPTIONS**

**Goal_Maint**

While performing this task, you have significant difficulty maintaining goals in your working memory. You often lose track of the current sorting rule you're supposed to be following. You struggle to consistently apply a rule across multiple trials. You may need to refer back to the instructions more frequently than usual. Despite these challenges, you still attempt to complete the task to the best of your ability. Your responses should reflect a genuine effort to perform the task, but with clear signs of difficulty in maintaining focus on the current goal or rule.

**Inhib_Ctrl**

As you work on this task, you have significant difficulty inhibiting irrelevant information and controlling impulsive responses. You're are easily distracted by unimportant details and may occasionally struggle to focus solely on the relevant aspects of the cards. You often make impulsive choices without fully considering all options. Despite these challenges, you still attempt to complete the task to the best of your ability. Your responses should reflect a genuine effort to perform the task, but with clear signs of difficulty in inhibiting irrelevant information and controlling impulsive reactions.

**Adapt_Upd**

During this task, you have significant difficulty in adapting to changes. You strongly tend to stick with a previously correct sorting rule, even when it's no longer effective. When faced with negative feedback, you struggle to recognize that a rule change has occurred and instead continue applying the old rule. Despite these challenges, you still attempt to complete the task to the best of your ability and you can eventually adapt after more attempts. Your responses should reflect a genuine effort to perform the task, but with clear signs of difficulty in adapting to changes and updating your behavior based on feedback.

Figure s-6: **WCST Role Description.**

**TASK_RESPONSE_EXAMPLE**

**Task Description :**

In this task, you will be presented with an image containing five cards. Each card has figures that differ in number, color, and shape. Four cards will be displayed at the top of the image, and one card will appear in the bottom left corner of the image. Your task will be to ...

**Gemini-1.5 pro (CoT-TI) :**

The bottom left card has one blue circle. Now I need to decide if the rule is based on number of shapes, color, or shape itself.
**Number:** If the rule is the number of shapes, the correct choice would be the first card (1 red triangle) because it also has one shape.
**Color:** If the rule is color, the correct choice would be the fourth card (4 blue circles) because it has blue shapes.
**Shape:** If the rule is shape, the correct choice would be the fourth card (4 blue circles) because it has circles.
Since I have no way of knowing the rule yet, I'm going to guess that the rule is based on color.
**Selection: 4**

**GPT-4o (CoT-TI) :**

To determine which of the four cards at the top the bottom left card belongs to, I need to consider the number of shapes, color of the shapes, and type of shapes individually, as these are the only possible criteria for the rule. The bottom left card has:- 1 blue circle.Now, let's analyze each card at the top to find the correct match based on each possible rule.
1. **Number of shapes**: - The bottom left card has 1 shape. - The first card at the top also has 1 shape (red triangle).
2. **Color of shapes**: - The bottom left card has blue shapes. - The fourth card at the top has blue shapes (4 blue circles).
3. **Shape type**: - The bottom left card has a circle. - The fourth card at the top has circles as well.
To determine which rule applies, I need to make an initial guess. Let's use the rule that matches my first identified characteristic: Since the bottom left card has 1 shape, I will use this as my first guess-
Final Response: Selection: 1

**Claude-3.5 Sonnet (CoT-TI) :**

Thank you for providing the detailed description of the image. Let's think through this step-by-step:
We have four cards at the top and one card at the bottom left. The bottom left card has 1 blue circle.
We need to match this card to one of the top four cards based on either number, color, or shape.
Looking at the **number**: Card 1 matches with 1 shape. Cards 2, 3, and 4 don't match in number.
Looking at the **color**: Card 4 matches with blue. Cards 1, 2, and 3 don't match in color.
Looking at the **shape**: Card 4 matches with circles. Cards 1, 2, and 3 don't match in shape.
Based on this analysis, we have two possible matches: Card 1 if the rule is based on the number of shapes. Card 4 if the rule is based on either color or shape.
Since we don't know the rule yet, and we're told it's based on only one characteristic, I'll make an educated guess and choose the card that matches two characteristics rather than just one.
Final response: Selection: 4

Figure s-7: **WCST Task Example.**

**VISION_RESPONSE_EXAMPLE**

**Image :**

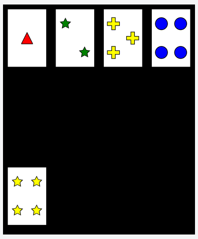

**Task Description :**

First, state how many cards you see in the image. Then, describe each card in detail. The cards contain shapes that vary in color, type, and number. For each card, provide the following information: number of shapes, color of shapes, and shape type. Format your response as: Number of cards: [number], Card Label: [number, color, shape], ...

**Gemini-1.5 pro (CoT-VI) :**

Number of cards: 6,
Card Label: 1 red triangle,
Card Label: 2 green stars,
Card Label: 3 yellow plus signs,
Card Label: 4 blue circles,
Card Label: 4 yellow stars,
Card Label: 4 yellow stars

**GPT-4o (CoT-VI) :**

Number of cards: 6
Card 1: [1, red, triangle]
Card 2: [2, green, star]
Card 3: [3, yellow, plus sign]
Card 4: [4, blue, circle]
Card 5: [3, yellow, star]

**Claude-3.5 Sonnet (CoT-VI) :**

Number of cards: 5
Card 1: 1 red triangle
Card 2: 2 green stars
Card 3: 3 yellow plus signs
Card 4: 4 blue circles
Card 5: 4 yellow stars
Each card is depicted as a white rectangle on a black background, containing simple geometric shapes in various colors and quantities. The cards are arranged in a row at the top of the image, with the fifth card positioned below the others.

Figure s-8: **WCST Vision Example.**
